# Supplementary material for: Learning Ising models from one or multiple samples
Source: arXiv:2004.09370 source file (2020-12-10)
Supplement: Supplementary file 1 [file additional-examples.tex]

\section{Additional examples}
\label{app:addnl-examples}

\subsection{Multiple networks, each containing sufficiently many unique friendships}

Here is an example when the theorem can be applied: assume we have $k$ different types of connections, corresponding to graphs $([n],E_1),\dots,([n],E_k)$ with incidence matrices $J^1,\dots,J^k$, namely, $J^{s}_{ij} = 1$ if $(i,j) \in E_s$ and otherwise $J^s_{ij} = 0$. 
Assume that each connection graph has an unknown influence $\beta_i$, such that the interaction matrix of the Ising model is $J^* = \sum_i \beta_i^* J^i$. For all $s$, let
\[
\Lambda_s = E_s \setminus (\bigcup_{t \in [n]\setminus\{s\}} E_t),
\]
and let $\lambda_s = |\Lambda_s|$ which equals the number of edges unique to $E_s$.
Assume that $\hat J = \sum_s \hat\beta_s J^s$. Then,
\[
\sum_s \lambda_s (\hat\beta_s - \beta_s^*)^2 \le \|\hat J - J^*\|_F^2,
\]
and particularly,
\[
\|\hat \beta_s - \beta_s^*\|_2
\le \frac{\|\hat J - J^*\|_F}{\sqrt{\min_s \lambda_s}}.
\]

To prove the above, we substitute $\beta:=\hat\beta - \beta^*$ and calculate
\[
\|\sum_s \beta_s J^s\|_F^2 
= \sum_{i,j\in[n]}(\sum_{s\in[k]} \beta_s J^s_{ij})^2
\ge \sum_{i,j\in[n]}\sum_{s \in [k]} \sum_{(i,j) \in \Lambda_s}\beta_s^2
= \sum_s \lambda_s \beta_s^2.
\]

\subsection{Samples from a network with an additional temporal correlation}

\section{Can we get a tight bound on the partition function?}
We essentially have to compare $x^\top A x$ and $x^\top A^2 x$. Decompose into the singular values...

Use the result from inference in Ising models, where they compare $x$ to $Ax$, and in fact say that $x \approx \tanh (Ax)$.

Perhaps replace the maximum over sub-samples by a simple bound of $\|Ax\|_2 + 1$. We actually already have this: the derivative is bounded in terms of the value of $\|Ax\|_2$. By the triangle inequality and using their trick, we get that $x^\top A x$ cannot be much larger than $x^\top A^\top A x$.

So, in fact, we get a control as a function of $x^\top A x$: if it's large then we can learn, and otherwise, we cannot!

Rate can be \emph{certified} by $x^\top A x$: if this value is large, then we know that we've learned well! Even if we don't have the guarantee on the partition function, that was needed in "inference".

Have an improved statement over inference, that only requires one sided bound on the partition function.

Say we have one matrix $J$ and that the true parameter is $\beta^*$. Let $F(\beta)$ denote the log partition function.

We have the following lemma:
\begin{lemma}
	
\end{lemma}
\begin{proof}
	First of all, let $J$ denote the true matrix.
	And $r > 0$. Then, we have that
	\[
	\Pr_{J}[x^\top J x < r]
	= \Pr[e^{-x^\top J x/2} < e^{-r/2}]
	\le \exp(\frac{1}{2}r - F_n(J))
	\]
	Next, we compare $x^\top J x$ with $x^\top J^\top J x$, and show that $x^\top J^\top J x \ge C x^\top J x$. Indeed, assume that $x^\top J x \ge x^\top J^\top J x$, otherwise we're done. Then, we derive that $x^\top J^\top J x \ge \tanh(x^\top J^\top) J x$, since in the inner product we have a sum of $n$ products, and in each one of them we have an inequality. Next, we have that 
	\[
	|\tanh(x^\top J^\top) J x - x^\top J x| \le C \|Jx\|_2,
	\]
	from the above inequality. We derive that
	\[
	\|Jx\|_2^2 
	\ge |\tanh(x^\top J^\top) Jx| 
	\ge |x^\top J x| - \|Jx\|_2.
	\]
	We have an inequality: $x^2 + x - t \ge 0$, hence we derive that the solution are
	\[
	\frac{-1\pm \sqrt{1+4t}}{2}.
	\]
	Since we have the positive inequality, we get that $\|Jx\|_2 \ge \Omega(-1 + \sqrt{1+4t})$.
	
	So, we derive that the strong convexity is at least $x^\top J x$, namely, $\partial^2\varphi(J)/\partial J^2 \ge F_n(J)/2$. And the derivative is a square root of that. Therefore, $\|\hat{J} - J\| \le \sqrt{1/F_n} \|J\|$.
	Now, in terms of $\beta$, it means that the rate is bounded by $\beta^* /\sqrt{F_n}$.
	
	Notice what happens under Dobrushin's condition with a small $\beta$. In the Frobenius shape, the error would be $1/\|J\|_F$. The partition function is $F(A) = \|A\|_F^2$, hence for our case it is $\beta^2 \|J\|_F^2$. And, if we take $\beta / \|A\|_F^2$, we have $1/\sqrt{\|J\|_F}$.
\end{proof}
\yuval{If we can show that the partition function is lower bounded by the Frobenius norm, then we can show that our theorem is tight under Dobrushin's condition. Additionally, this will show that the Frobenius lower bound is weaker than the partition function bound. Indeed, this is true because we can learn up to a rate of $1/\|A\|_F$ under Dobrushin's condition, and otherwise it wouldn't be possible! Also we can check the proof of inference in Ising models.}

Can we lower bound the partition function by the Frobenius norm? Use the variance of $x^\top A x$.

\yuval{Find specific applications. For example, Curie Weiss (although it's known), or, random graph in high temperature.}

\subsection{One parameter}

In the one-parameter setting, using the same proof as Theorem\yuval{REF- multi-parameters}, we can perform a more fine-grained analysis. Here we assume a known interaction matrix $J \in M_{n\times n}(\mathbb{R})$ and an unknown parameter $\beta^*$, such that $x \sim P_{\beta^* J}$. As in Theorem\yuval{REF} we assume that $\|\beta^*J\|_\infty$ is at most some constant, and without loss of generality, $\|J\|_\infty = 1$ and $\beta^* = O(1)$ (possibly $\beta > 1$). We analyze the pseudo log likelihood estimator:
\begin{theorem}[informal]
	Assume that $\|J\|_\infty = 1$, and let $\hat \beta$ denote the pseudo likelihood estimator of $\beta^*$. Then, with high probability over $x$,
	\[
		|\hat\beta-\beta^*|
		\le O(\|Jx\|_2^{-1} \sqrt{\log\log n})
		\le O(\beta^* Z_{\beta^*J}^{-1/2}\sqrt{\log\log n})
		\le O(\|J\|_F^{-1}\sqrt{\log \log n}).
	\]
\end{theorem}
We note that this nearly generalizes and improves all the prior work.
Chatterjee \yuval{cite} was the first to study this problem, and he gave a rate of $1/\sqrt{n}$ assuming that $Z_{\beta^*J} \ge $

\section{Parameter-specific learning}

\section{People to remember to cite}

Aryeh Kanterovich

Valiant?

Dheeraj
