# Supplementary material for: Learning Ising models from one or multiple samples
Source: arXiv:2004.09370 source file (2020-12-10)
Supplement: Supplementary file 2 [file temp-additional-lemmas.tex]

\section{Temporary additional lemmas}
